# Supplementary material for: BrainIB++: Leveraging Graph Neural Networks and Information Bottleneck for Functional Brain Biomarkers in Schizophrenia
Source: arXiv:2510.03004 ancillary file (2025-10-03)
Supplement: Supplementary file 1 [file supplyment.pdf]

# Supplementary material for BrainIB++: Leveraging Graph Neural Networks and Information Bottleneck for Functional Brain Biomarkers in Schizophrenia

Tianzheng Hu, Qiang Li, Shu Liu, Vince D. Calhoun, Guido van Wingen, and Shujian Yu

## I. Quantitative Evaluation of Explanation

To further evaluate the interpretability of our model, we conducted a quantitative comparison with a widely used post-hoc explanation method, GNNExplainer [1], using a widely recognized dataset called MUTAG [2]. The MUTAG dataset consists of 188 chemical compounds represented as graphs, where nodes correspond to atoms (e.g., carbon, nitrogen, oxygen) and edges represent chemical bonds (e.g., single, double, aromatic bonds). Each compound is labeled as either mutagenic or non-mutagenic based on its ability to induce genetic mutations in Salmonella typhimurium.

To enable quantitative evaluation of explanation quality, we manually annotated substructures that are widely known to be associated with mutagenic activity as ground truth for model explanation. Specifically, these functional groups include nitro groups ($NO_2$), aromatic amines ($NH_2$ attached to aromatic rings), and certain heterocycles, which have been empirically linked to increased mutagenicity in prior biochemical studies [3], [4]. We compared the substructures identified by GNNExplainer and BrainIB++ against the ground-truth functional groups obtained in the previous step. This comparison enabled the use of standard confusion matrix-based metrics, including accuracy, precision, recall, and F1 score, to quantitatively evaluate how well the generated explanations aligned with the ground truth (see Table I).

TABLE I: Quantitative analysis of explanation results for GNNExplainer and BrainIB++ with MUTAG dataset.

| Model | Accuracy | Precision | Recall | F1 score |
|---|---|---|---|---|
| GNNExplainer | 0.6269 | **0.7943** | 0.5294 | 0.6160 |
| BrainIB++ | **0.9106** | 0.7617 | **0.9785** | **0.8457** |

The GNNExplainer achieves a relatively modest performance with 0.6269 accuracy, 0.7943 precision, 0.5294 recall, and an F1 score of 0.6160. While it provides post-hoc explanations by identifying relevant subgraphs for a given prediction, its reliance on gradient-based masking often leads to limited generalization across different graph structures and fails to capture broader substructure semantics.

In contrast, our BrainIB++ model achieves consistently strong performance across all metrics, with 0.9106 accuracy, 0.7617 precision, 0.9785 recall, and an F1 score of 0.8457. These results highlight that our built-in interpretability mechanism not only identifies highly relevant substructures but also does so with superior coverage and precision. Unlike post-hoc interpretation methods such as GNNExplainer, which often face challenges in accurately attributing edge and node importance and exhibit limited generalizability across different data modes, BrainIB++ offers intrinsically faithful and task-aligned explanations derived directly from its subgraph-based decision process.

This suggests that integrating interpretability into the model architecture rather than opposed to relying on external explainers yields more reliable and comprehensive explanations, particularly in chemistry-related tasks where substructure identification is critical.

## II. Statistical Analysis

### A. Global topological metrics with FDR

We conducted group comparisons across all global and nodal metrics using two-sample t-tests, followed by Benjamini-Hochberg procedure false discovery rate (FDR) correction. Table II and III report the global and nodal metrics that showed statistically significant differences after FDR correction.

TABLE II: Group comparison of global topological metrics between patients and controls in BSNIP (with FDR correction). Bold p-values indicate statistical significance.

| **Metric** | **T-value** | **p-value** | **FDR p-value** | **Significance** |
|---|---|---|---|---|
| Average Degree | -0.884 | 0.377 | 0.427 | Not significant |
| Average Clustering | 0.795 | 0.426 | 0.427 | Not significant |
| Global Efficiency | -2.451 | **0.014** | **0.043** | **Significant** |

TABLE III: Group comparison of nodal topological metrics between patients and controls in BSNIP (with FDR correction). SZ and HC denote subjects with schizophrenia and health control, respectively.

| **Brian Region** | **Degree** | | **Efficiency** | | **Betweenness** | | **p-value** | | | **FDR p-value** | | |
|---|---|---|---|---|---|---|---|---|---|---|---|---|
| | HC | SZ | HC | SZ | HC | SZ | Degree | Efficiency | Betweenness | Degree | Efficiency | Betweenness |
| Frontal_Mid_Orb_L | 3.778 | 3.229 | 0.406 | 0.390 | 0.012 | 0.008 | 0.005 | 0.497 | 1.00E-05 | 0.065 | 0.825 | **0.001** |
| Occipital_Sup_L | 7.948 | 7.114 | 0.809 | 0.770 | 0.011 | 0.011 | 0.0001 | 0.009 | 0.649 | **0.010** | 0.196 | 0.874 |
| Hippocampus_L | 5.041 | 5.622 | 0.537 | 0.528 | 0.018 | 0.029 | 0.047 | 0.687 | 3.00E-05 | 0.174 | 0.95453 | **0.001** |

At the global level, a significant group difference in global efficiency was observed and remained after correction (see Table II). However, at the nodal level, no regions selected by BrainIB++ survived after correction despite a few showing uncorrected differences (see Table III). Specifically, three regions emerged: the left superior occipital gyrus (Degree), the left middle orbital frontal gyrus (Betweenness), and the left hippocampus (Betweenness). These regions are linked to visual processing, emotional regulation, and memory functional domains frequently implicated in schizophrenia. This lack of significant univariate effects after correction is expected in psychiatric neuroimaging due to high inter-subject variability and subtle effect sizes.

This observation underscores the value of multivariate approaches. Traditional univariate tests struggle to detect distributed, overlapping alterations, while our BrainIB++ model leverages complementary network-level features to capture broader, biologically meaningful patterns of disruption that may be individually weak but collectively informative. As such, multivariate machine learning methods provide powerful tools for individual-level prediction, beyond what univariate statistics alone can reveal [5].

### *B. Statistical analysis for UCLA and COBRE dataset*

We have now performed additional node-level statistical analyses for the UCLA and COBRE datasets (see Table IV and Table V). The results show that very few brain regions exhibit significant group differences (e.g., only Supp_Motor_Area_L in COBRE for Degree, with $p = 0.039$), while the majority of comparisons are non-significant ( $p > 0.05$). This further supports our original assessment that the smaller sample sizes in these datasets limit the statistical power to detect robust effects, except for potentially large-magnitude differences. The consistency of these findings with the BSNIP results (where more significant differences were identified, which might be due to a larger $N$) reinforces the importance of sample size in such analyses.

TABLE IV: Group comparison of node topological metrics between patients and controls in UCLA. Bold p-values indicate statistical significance.

| **BrianIB++** | **Degree** | | **Efficiency** | | **Betweenness** | | **p Value** | | |
|---|---|---|---|---|---|---|---|---|---|
| | HC | SZ | HC | SZ | HC | SZ | Degree | Efficiency | Betweenness |
| Cuneus_L | 16.600 | 16.307 | 0.802 | 0.787 | 0.023 | 0.019 | 0.799 | 0.517 | 0.870 |
| Fusiform_R | 11.240 | 13.719 | 0.804 | 0.809 | 0.013 | 0.018 | 0.243 | 0.942 | 0.248 |
| Occipital_Inf_L | 19.460 | 16.632 | 0.684 | 0.681 | 0.032 | 0.026 | 0.323 | 0.942 | 0.200 |
| Occipital_Inf_R | 16.260 | 15.711 | 0.837 | 0.799 | 0.016 | 0.019 | 0.767 | 0.135 | 0.248 |
| Supp_Motor_Area_L | 17.900 | 16.009 | 0.808 | 0.788 | 0.012 | 0.015 | 0.323 | 0.592 | 0.248 |
| Calcarine_L | 22.580 | 20.667 | 0.776 | 0.736 | 0.031 | 0.030 | 0.323 | 0.086 | 0.871 |
| Postcentral_R | 11.280 | 8.640 | 0.671 | 0.526 | 0.015 | 0.012 | 0.323 | **0.049** | 0.463 |
| Calcarine_R | 9.380 | 7.816 | 0.617 | 0.531 | 0.033 | 0.023 | 0.323 | 0.170 | 0.248 |
| Postcentral_L | 9.020 | 10.904 | 0.717 | 0.769 | 0.033 | 0.018 | 0.268 | 0.170 | 0.200 |
| **SVM** | **Degree** | | **Efficiency** | | **Betweenness** | | **p Value** | | |
| | HC | SZ | HC | SZ | HC | SZ | Degree | Efficiency | Betweenness |
| Amygdala_R | 17.260 | 16.474 | 0.810 | 0.787 | 0.017 | 0.021 | 0.649 | 0.295 | 0.249 |
| Caudate_R | 12.340 | 12.325 | 0.791 | 0.774 | 0.013 | 0.016 | 0.992 | 0.360 | 0.249 |
| Calcarine_L | 22.580 | 20.667 | 0.776 | 0.736 | 0.031 | 0.030 | 0.323 | 0.086 | 0.871 |
| Postcentral_R | 11.280 | 8.640 | 0.671 | 0.526 | 0.015 | 0.012 | 0.305 | **0.027** | 0.463 |
| Calcarine_R | 9.380 | 7.816 | 0.617 | 0.531 | 0.033 | 0.023 | 0.326 | 0.116 | 0.249 |
| Postcentral_L | 9.020 | 10.904 | 0.717 | 0.769 | 0.033 | 0.018 | 0.292 | 0.116 | 0.200 |

## III. Supplement of feature calculation

Given a graph $G = (V, E)$ where $V$ is the set of vertices (nodes) and $E$ is the set of edges, the features can be calculated as follow:

*a)* ***Edges:*** The number of edges $|E|$ in a graph is simply the count of edges.

*b)* ***Degree:*** The degree $d(v)$ of a vertex $v$ is the number of edges connected to $v$.

TABLE V: Group comparison of node topological metrics between patients and controls in COBRE. Bold p-values indicate statistical significance.

| **BrianIB++** | **Degree** | | **Efficiency** | | **Betweenness** | | **p Value** | | |
|---|---|---|---|---|---|---|---|---|---|
| | HC | SZ | HC | SZ | HC | SZ | Degree | Efficiency | Betweenness |
| Cuneus_L | 12.094 | 12.234 | 0.794 | 0.758 | 0.020 | 0.022 | 0.959 | 0.509 | 0.985 |
| Fusiform_R | 27.906 | 28.000 | 0.879 | 0.864 | 0.009 | 0.012 | 0.959 | 0.336 | 0.823 |
| Occipital_Inf_L | 21.500 | 16.532 | 0.813 | 0.742 | 0.044 | 0.092 | 0.136 | 0.113 | 0.101 |
| Occipital_Inf_R | 15.438 | 18.064 | 0.858 | 0.822 | 0.019 | 0.020 | 0.472 | 0.394 | 0.985 |
| Supp_Motor_Area_L | 19.969 | 13.745 | 0.866 | 0.809 | 0.006 | 0.005 | **0.039** | 0.348 | 0.985 |
| Calcarine_R | 11.875 | 7.404 | 0.551 | 0.441 | 0.040 | 0.026 | 0.168 | 0.336 | 0.823 |
| Postcentral_L | 7.719 | 7.319 | 0.647 | 0.501 | 0.030 | 0.029 | 0.959 | 0.204 | 0.985 |
| Postcentral_R | 7.625 | 5.128 | 0.618 | 0.386 | 0.003 | 0.005 | 0.330 | 0.113 | 0.823 |
| **SVM** | **Degree** | | **Efficiency** | | **Betweenness** | | **p Value** | | |
| | HC | SZ | HC | SZ | HC | SZ | Degree | Efficiency | Betweenness |
| Amygdala_R | 31.344 | 31.191 | 0.851 | 0.827 | 0.020 | 0.025 | 0.886 | 0.126 | 0.539 |
| Caudate_R | 11.938 | 9.532 | 0.778 | 0.670 | 0.014 | 0.025 | 0.270 | 0.061 | 0.143 |
| Calcarine_L | 18.688 | 14.170 | 0.745 | 0.620 | 0.022 | 0.035 | 0.229 | 0.061 | 0.477 |
| Calcarine_R | 11.875 | 7.404 | 0.551 | 0.441 | 0.040 | 0.026 | 0.168 | 0.336 | 0.823 |
| Postcentral_L | 7.719 | 7.319 | 0.647 | 0.501 | 0.030 | 0.029 | 0.959 | 0.204 | 0.985 |
| Postcentral_R | 7.625 | 5.128 | 0.618 | 0.386 | 0.003 | 0.005 | 0.330 | 0.113 | 0.823 |

*c)* ***Degree Centrality:*** The degree centrality $C_D(v)$ of a vertex $v$ is defined as:

$$C_D(v) = \frac{d(v)}{|v| - 1} \tag{1}$$

, where $d(v)$ is the degree of vertex $v$, and $|V|$ is the number of vertices in the graph.

*d)* ***Betweenness Centrality:*** The betweenness centrality $C_B(v)$ of a vertex $v$ is defined as:

$$C_B(v) = \sum_{s \neq v \neq t} \frac{\sigma_{st}(v)}{\sigma_{st}} \tag{2}$$

, where $\sigma_{st}$ is the total number of shortest paths from vertex $s$ to vertex $t$ and $\sigma_{st}(v)$ is the number of those paths that pass through $v$.

*e)* ***Closeness Centrality:*** The closeness centrality $C_C(v)$ of a vertex $v$ is defined as:

$$C_C(v) = \frac{|V| - 1}{\sum_{u \in V} d(v, u)} \tag{3}$$

, where $d(v, u)$ is the shortest path distance between vertices $v$ and $u$ .

*f)* ***Load Centrality:*** Load centrality $C_L(v)$ measures the fraction of all shortest paths that pass through a given node. It is similar to betweenness centrality but is weighted by the total number of shortest paths through the network:

$$C_L(v) = \sum_{i \neq v \neq j} \frac{\sigma_{ij}(v)}{\sigma_{ij}} \tag{4}$$

, where $\sigma_{ij}$ is the total number of shortest paths between nodes $i$ and $j$, $\sigma_{ij}(v)$ is the number of those shortest paths that pass through node $v$.

*g)* ***Average Shortest Path Length:*** The average shortest path length $l$ of a given node is defined as:

$$L_v = \frac{1}{N - 1} \sum_{i \neq v} d(v, i) \tag{5}$$

, where $d(v, i)$ is the shortest path distance between vertices $v$ and $i$.

*h)* ***Average Neighbor Degree:*** The average neighbor degree $K_{avg}(v)$ of a vertex $v$ is defined as:

$$K_{avg}(v) = \frac{1}{d(v)} \sum_{u \in N(v)} d(u) \tag{6}$$

, where $N(v)$ is the set of neighbors of $v$ and $d(u)$ is the degree of neighbor $u$.

*i)* ***Global Average Shortest Path Length:*** The global average shortest path length $l$ of a graph is defined as:

$$l = \frac{1}{|V|(|V| - 1)} \sum_{s \neq t} d(s, t) \tag{7}$$

, where $d(s, t)$ is the shortest path distance between vertices $s$ and $t$.

*j) **Global Average Degree:*** The global average degree $k$ can be expressed mathematically as:

$$k = \frac{1}{N} \sum_{i=1}^{N} k_i, \tag{8}$$

, where $N$ is the total number of nodes in the graph and $k_i$ is the degree of node $i$.

## IV. The mapping table between Group ICA Networks and AAL

TABLE VI: The mapping of Independent Component Analysis (ICA) networks to the Automated Anatomical Labeling (AAL) parcellation is detailed as follows. The **ID** denotes the identification number of each brain networks from the Group ICA, which encompasses a total of 105 ICNs. The **X**, **Y**, and **Z** values represent the spatial coordinates of the ICA brain networks. The **Label** indicates the functional network to which each ICN belongs, including the Cerebellar network, Higher Cognition network, Sensorimotor network, Subcortical network, Temporal network, and Visual network. The **1st**, **2nd**, and **3rd** columns list the AAL parcellation brain regions with the three shortest distances to the corresponding ICA networks. **Region 1, 2, and 3** are the abbreviated names of these regions. In this study, we selected the nearest brain region (denoted as **1st Distance**) as the corresponding brain region for the interpretable explanation.

| ID | X | Y | Z | Label | 1st | Region 1 | 2nd | Region 2 | 3rd | Region 3 |
|---|---|---|---|---|---|---|---|---|---|---|
| 5 | 21 | -67 | -31 | Cerebellar | 11.96 | CRBL6.R | 14.37 | CRBLCrus2.R | 16.52 | CRBLCrus1.R |
| 18 | 0 | -52 | -19 | Cerebellar | 12.95 | Vermis45 | 13.27 | Vermis12 | 14.12 | Vermis10 |
| 23 | 15 | -46 | -22 | Cerebellar | 5.43 | CRBL45.R | 12.12 | CRBL3.R | 15.76 | CRBL6.R |
| 30 | -27 | -58 | -40 | Cerebellar | 7.86 | CRBL7b.L | 8.52 | CRBL8.L | 15.45 | CRBLCrus2.L |
| 31 | 30 | -55 | -43 | Cerebellar | 8.25 | CRBL8.R | 10.32 | CRBL7b.R | 14.50 | CRBLCrus2.R |
| 33 | -15 | -46 | -25 | Cerebellar | 8.45 | CRBL45.L | 12.52 | CRBL3.L | 15.74 | CRBL6.L |
| 47 | 39 | -40 | -40 | Cerebellar | 14.46 | CRBL10.R | 20.47 | FFG.R | 23.47 | CRBL8.R |
| 56 | -21 | -55 | -52 | Cerebellar | 6.44 | CRBL8.L | 13.22 | CRBL9.L | 13.97 | CRBL7b.L |
| 73 | -3 | -64 | -16 | Cerebellar | 5.22 | Vermis6 | 12.79 | Vermis7 | 15.85 | Vermis45 |
| 91 | 30 | -82 | -37 | Cerebellar | 13.47 | CRBLCrus2.R | 18.22 | CRBLCrus1.R | 22.26 | CRBL7b.R |
| 92 | -3 | -61 | -31 | Cerebellar | 6.20 | Vermis8 | 8.23 | Vermis9 | 13.08 | Vermis7 |
| 94 | 12 | -55 | -52 | Cerebellar | 8.30 | CRBL9.R | 13.37 | CRBL8.R | 20.41 | Vermis9 |
| 99 | 0 | -49 | -13 | Cerebellar | 7.76 | Vermis45 | 9.31 | Vermis3 | 12.43 | Vermis12 |
| 2 | 0 | 50 | 20 | Higher Cognition | 11.93 | SFGmed.L | 13.71 | SFGmed.R | 16.05 | ACG.R |
| 4 | -48 | 20 | 23 | Higher Cognition | 8.30 | IFGoperc.L | 13.61 | IFGtriang.L | 23.01 | MFG.L |
| 6 | -9 | -67 | 35 | Higher Cognition | 15.57 | CUN.L | 17.08 | PCUN.L | 20.04 | SOG.L |
| 8 | -24 | 50 | -7 | Higher Cognition | 7.16 | ORBmid.L | 10.12 | ORBsup.L | 19.27 | ORBsupmed.L |
| 9 | -51 | -46 | -7 | Higher Cognition | 13.87 | MTG.L | 24.19 | ITG.L | 24.52 | FFG.L |
| 11 | -30 | 62 | 8 | Higher Cognition | 21.09 | ORBmid.L | 29.16 | ORBsup.L | 30.28 | ORBsupmed.L |
| 24 | -12 | -52 | 11 | Higher Cognition | 17.90 | PCG.L | 21.63 | Vermis45 | 22.21 | LING.L |
| 26 | -60 | -40 | 41 | Higher Cognition | 13.02 | SMG.L | 19.04 | IPL.L | 25.92 | PoCG.L |
| 32 | 0 | 35 | 11 | Higher Cognition | 5.02 | ACG.L | 9.95 | ACG.R | 24.89 | SFGmed.L |
| 36 | -36 | 14 | 29 | Higher Cognition | 15.99 | IFGoperc.L | 19.98 | MFG.L | 23.88 | IFGtriang.L |
| 39 | -48 | 26 | 5 | Higher Cognition | 10.10 | IFGtriang.L | 19.31 | IFGoperc.L | 21.43 | ORBinf.L |
| 44 | 51 | -46 | 14 | Higher Cognition | 18.92 | MTG.R | 25.95 | SMG.R | 26.26 | STG.R |
| 51 | -9 | 8 | 62 | Higher Cognition | 4.88 | SMA.L | 19.28 | SMA.R | 30.90 | DCG.L |
| 52 | -15 | 11 | 53 | Higher Cognition | 14.20 | SMA.L | 26.37 | SFGdor.L | 27.45 | SMA.R |
| 53 | -48 | -46 | 8 | Higher Cognition | 17.59 | MTG.L | 25.86 | STG.L | 26.79 | SMG.L |
| 55 | 51 | 23 | 17 | Higher Cognition | 7.73 | IFGtriang.R | 9.19 | IFGoperc.R | 23.90 | MFG.R |
| 57 | -45 | 20 | 23 | Higher Cognition | 8.97 | IFGoperc.L | 13.41 | IFGtriang.L | 21.24 | MFG.L |
| 58 | 48 | -43 | 8 | Higher Cognition | 14.58 | MTG.R | 23.55 | STG.R | 26.05 | HES.R |
| 59 | -6 | -55 | 50 | Higher Cognition | 2.58 | PCUN.L | 17.18 | PCUN.R | 20.14 | SPG.L |
| 60 | -12 | -58 | 20 | Higher Cognition | 17.33 | PCG.L | 24.06 | CUN.L | 25.19 | CAL.L |
| 62 | 0 | 32 | 20 | Higher Cognition | 8.03 | ACG.L | 10.68 | ACG.R | 20.89 | SFGmed.L |
| 63 | 57 | -46 | 23 | Higher Cognition | 18.50 | SMG.R | 23.91 | ANG.R | 26.00 | MTG.R |
| 65 | -51 | -58 | 41 | Higher Cognition | 9.18 | ANG.L | 15.77 | IPL.L | 26.98 | SMG.L |
| 68 | 48 | -58 | 47 | Higher Cognition | 8.95 | ANG.R | 12.08 | IPL.R | 26.60 | SPG.R |
| 69 | -45 | -61 | 50 | Higher Cognition | 14.44 | ANG.L | 15.68 | IPL.L | 23.38 | SPG.L |

| ID | X | Y | Z | Label | 1st | Region 1 | 2nd | Region 2 | 3rd | Region 3 |
|---|---|---|---|---|---|---|---|---|---|---|
| 81 | 48 | -64 | 38 | Higher Cognition | 4.77 | ANG.R | 21.19 | IPL.R | 26.54 | MOG.R |
| 83 | 0 | 47 | 35 | Higher Cognition | 6.68 | SFGmed.L | 10.97 | SFGmed.R | 23.21 | ACG.R |
| 85 | 33 | 23 | -4 | Higher Cognition | 14.67 | ORBinf.R | 18.81 | INS.R | 19.91 | PUT.R |
| 86 | 51 | 20 | 17 | Higher Cognition | 6.73 | IFGoperc.R | 10.57 | IFGtriang.R | 23.56 | INS.R |
| 87 | -48 | -64 | 35 | Higher Cognition | 5.04 | ANG.L | 22.26 | IPL.L | 29.67 | MOG.L |
| 88 | 0 | 41 | 2 | Higher Cognition | 13.80 | ACG.L | 16.24 | ORBsupmed.R | 16.70 | ACG.R |
| 10 | 36 | -10 | 41 | Sensorimotor | 12.45 | PreCG.R | 20.07 | PoCG.R | 28.03 | DCG.R |
| 34 | -54 | -25 | 38 | Sensorimotor | 11.61 | SMG.L | 16.06 | PoCG.L | 25.21 | IPL.L |
| 41 | 0 | -1 | 59 | Sensorimotor | 8.26 | SMA.L | 9.15 | SMA.R | 22.24 | DCG.R |
| 43 | 54 | -22 | 29 | Sensorimotor | 11.55 | SMG.R | 20.87 | HES.R | 21.36 | ROL.R |
| 49 | 60 | -25 | 41 | Sensorimotor | 9.51 | SMG.R | 21.87 | PoCG.R | 26.64 | IPL.R |
| 70 | -9 | 2 | 44 | Sensorimotor | 17.45 | DCG.L | 17.99 | SMA.L | 20.61 | DCG.R |
| 71 | 0 | -25 | 65 | Sensorimotor | 9.17 | PCL.L | 10.44 | PCL.R | 26.09 | DCG.L |
| 96 | 21 | -25 | 59 | Sensorimotor | 17.57 | PCL.R | 21.43 | PoCG.R | 27.29 | PreCG.R |
| 98 | -15 | -10 | 62 | Sensorimotor | 17.74 | SMA.L | 18.85 | PCL.L | 23.07 | DCG.L |
| 100 | 21 | -52 | 71 | Sensorimotor | 12.55 | SPG.R | 24.65 | PCL.R | 29.65 | PCUN.R |
| 102 | 39 | -22 | 59 | Sensorimotor | 7.73 | PoCG.R | 15.61 | PreCG.R | 27.11 | IPL.R |
| 104 | -39 | -22 | 62 | Sensorimotor | 13.54 | PoCG.L | 19.72 | PreCG.L | 28.54 | IPL.L |
| 105 | -51 | -10 | 32 | Sensorimotor | 18.52 | ROL.L | 22.78 | PoCG.L | 23.02 | PreCG.L |
| 3 | -21 | 5 | 5 | Subcortical | 4.07 | PUT.L | 7.67 | PAL.L | 12.04 | CAU.L |
| 13 | 42 | 5 | -13 | Subcortical | 12.21 | TPOsup.R | 15.42 | INS.R | 15.96 | AMYG.R |
| 14 | 6 | -13 | -4 | Subcortical | 14.69 | THA.R | 20.56 | PAL.R | 21.17 | THA.L |
| 15 | 21 | -13 | -1 | Subcortical | 12.94 | THA.R | 13.24 | PAL.R | 14.17 | HIP.R |
| 25 | 9 | 8 | -7 | Subcortical | 9.10 | OLF.R | 16.19 | PAL.R | 17.90 | CAU.R |
| 27 | 18 | 14 | -7 | Subcortical | 8.89 | OLF.R | 15.92 | PAL.R | 16.36 | PUT.R |
| 29 | 9 | -7 | 8 | Subcortical | 11.28 | THA.R | 16.15 | PAL.R | 19.99 | CAU.R |
| 35 | -36 | 5 | 11 | Subcortical | 7.79 | INS.L | 14.88 | PUT.L | 16.69 | IFGoperc.L |
| 38 | -27 | 2 | -4 | Subcortical | 7.35 | PUT.L | 10.36 | PAL.L | 11.96 | INS.L |
| 45 | -21 | -13 | -1 | Subcortical | 12.63 | HIP.L | 13.43 | PAL.L | 14.30 | THA.L |
| 48 | 6 | -4 | -4 | Subcortical | 16.32 | PAL.R | 19.46 | THA.R | 21.65 | OLF.R |
| 50 | 27 | 5 | -4 | Subcortical | 6.51 | PUT.R | 8.65 | PAL.R | 13.53 | INS.R |
| 54 | -3 | -13 | 2 | Subcortical | 10.87 | THA.L | 17.71 | THA.R | 19.72 | PAL.L |
| 61 | -39 | -31 | 14 | Subcortical | 13.11 | HES.L | 18.82 | STG.L | 23.31 | MTG.L |
| 76 | -18 | 11 | -10 | Subcortical | 10.83 | OLF.L | 14.66 | AMYG.L | 15.03 | PAL.L |
| 77 | 36 | -13 | 11 | Subcortical | 10.71 | HES.R | 18.33 | ROL.R | 21.43 | INS.R |
| 78 | 9 | -31 | 5 | Subcortical | 14.37 | THA.R | 20.10 | PCG.R | 20.17 | Vermis3 |
| 82 | -39 | -7 | 17 | Subcortical | 8.84 | ROL.L | 14.12 | HES.L | 19.63 | INS.L |
| 84 | 24 | 8 | -1 | Subcortical | 5.98 | PUT.R | 8.40 | PAL.R | 14.46 | CAU.R |
| 90 | -42 | -1 | -10 | Subcortical | 16.92 | INS.L | 19.20 | TPOsup.L | 20.05 | AMYG.L |
| 93 | 21 | 17 | 5 | Subcortical | 9.04 | CAU.R | 14.09 | PUT.R | 17.48 | PAL.R |
| 97 | -21 | 17 | 5 | Subcortical | 12.04 | CAU.L | 13.71 | PUT.L | 17.58 | INS.L |
| 101 | 63 | -25 | 5 | Subcortical | 6.09 | STG.R | 14.90 | MTG.R | 19.61 | HES.R |
| 1 | 24 | 2 | -34 | Temporal | 16.89 | AMYG.R | 21.89 | PHG.R | 23.86 | TPOmid.R |
| 12 | -24 | 8 | -25 | Temporal | 11.73 | AMYG.L | 16.66 | TPOmid.L | 18.07 | TPOsup.L |
| 37 | 21 | -7 | -25 | Temporal | 10.30 | PHG.R | 12.43 | AMYG.R | 21.13 | HIP.R |
| 40 | 30 | -31 | -4 | Temporal | 12.91 | HIP.R | 18.52 | FFG.R | 22.47 | CRBL45.R |
| 42 | 27 | 8 | -34 | Temporal | 18.07 | AMYG.R | 18.51 | TPOmid.R | 26.86 | PHG.R |
| 46 | -24 | 5 | -28 | Temporal | 12.27 | AMYG.L | 16.75 | TPOmid.L | 20.40 | TPOsup.L |
| 64 | 27 | 8 | -25 | Temporal | 10.51 | AMYG.R | 19.79 | TPOmid.R | 22.93 | OLF.R |
| 72 | 24 | -13 | -19 | Temporal | 2.95 | PHG.R | 12.19 | HIP.R | 14.12 | AMYG.R |
| 74 | -30 | -34 | -4 | Temporal | 15.43 | HIP.L | 17.45 | FFG.L | 21.96 | CRBL45.L |
| 75 | 27 | 5 | -37 | Temporal | 19.98 | AMYG.R | 20.26 | TPOmid.R | 26.11 | PHG.R |
| 79 | -21 | -7 | -25 | Temporal | 9.93 | PHG.L | 10.34 | AMYG.L | 20.64 | HIP.L |
| 80 | 51 | 14 | -25 | Temporal | 8.62 | TPOsup.R | 9.93 | TPOmid.R | 24.48 | ORBinf.R |
| 89 | -30 | 2 | -37 | Temporal | 14.39 | TPOmid.L | 21.14 | AMYG.L | 23.52 | TPOsup.L |
| 7 | -42 | -73 | -4 | Visual | 8.63 | IOG.L | 23.59 | MOG.L | 26.38 | CRBLCrus1.L |

| ID | X | Y | Z | Label | 1st | Region 1 | 2nd | Region 2 | 3rd | Region 3 |
|---|---|---|---|---|---|---|---|---|---|---|
| 16 | -9 | -94 | 26 | Visual | 12.51 | SOG.L | 14.26 | CUN.L | 24.92 | CAL.L |
| 17 | 45 | -61 | 5 | Visual | 24.81 | MOG.R | 25.42 | IOG.R | 27.61 | MTG.R |
| 19 | 30 | -49 | -10 | Visual | 14.74 | FFG.R | 16.37 | CRBL45.R | 17.36 | CRBL6.R |
| 20 | 30 | -73 | -1 | Visual | 13.82 | IOG.R | 15.27 | LING.R | 17.45 | CAL.R |
| 21 | 21 | -46 | -7 | Visual | 12.19 | CRBL45.R | 19.02 | CRBL3.R | 19.74 | FFG.R |
| 22 | -21 | -49 | -7 | Visual | 12.84 | CRBL45.L | 18.33 | CRBL6.L | 18.81 | FFG.L |
| 28 | -27 | -76 | -4 | Visual | 10.37 | IOG.L | 15.00 | LING.L | 21.35 | MOG.L |
| 66 | 27 | -94 | -4 | Visual | 16.79 | IOG.R | 27.12 | CAL.R | 29.11 | LING.R |
| 67 | 33 | -46 | -16 | Visual | 8.13 | FFG.R | 16.25 | CRBL45.R | 16.71 | CRBL6.R |
| 95 | -6 | -88 | -4 | Visual | 14.05 | CAL.L | 22.19 | LING.L | 24.76 | Vermis6 |
| 103 | 15 | -67 | 11 | Visual | 6.43 | CAL.R | 14.93 | LING.R | 21.26 | CUN.R |

## V. The AAL map

TABLE VII: The Automated Anatomical Labeling (AAL) parcellation map utilized in the BrainNet Viewer tool comprises a total of 116 brain regions. The **X**, **Y**, and **Z** values represent the spatial coordinates for each region.

| Index | X | Y | Z | Abbreviated Name | Name |
|---|---|---|---|---|---|
| 1 | -38.65 | -5.68 | 50.94 | PreCG.L | Precentral_L |
| 2 | 41.37 | -8.21 | 52.09 | PreCG.R | Precentral_R |
| 3 | -18.45 | 34.81 | 42.2 | SFGdor.L | Frontal_Sup_L |
| 4 | 21.9 | 31.12 | 43.82 | SFGdor.R | Frontal_Sup_R |
| 5 | -16.56 | 47.32 | -13.31 | ORBsup.L | Frontal_Sup_Orb_L |
| 6 | 18.49 | 48.1 | -14.02 | ORBsup.R | Frontal_Sup_Orb_R |
| 7 | -33.43 | 32.73 | 35.46 | MFG.L | Frontal_Mid_L |
| 8 | 37.59 | 33.06 | 34.04 | MFG.R | Frontal_Mid_R |
| 9 | -30.65 | 50.43 | -9.62 | ORBmid.L | Frontal_Mid_Orb_L |
| 10 | 33.18 | 52.59 | -10.73 | ORBmid.R | Frontal_Mid_Orb_R |
| 11 | -48.43 | 12.73 | 19.02 | IFGoperc.L | Frontal_Inf_Oper_L |
| 12 | 50.2 | 14.98 | 21.41 | IFGoperc.R | Frontal_Inf_Oper_R |
| 13 | -45.58 | 29.91 | 13.99 | IFGtriang.L | Frontal_Inf_Tri_L |
| 14 | 50.33 | 30.16 | 14.17 | IFGtriang.R | Frontal_Inf_Tri_R |
| 15 | -35.98 | 30.71 | -12.11 | ORBinf.L | Frontal_Inf_Orb_L |
| 16 | 41.22 | 32.23 | -11.91 | ORBinf.R | Frontal_Inf_Orb_R |
| 17 | -47.16 | -8.48 | 13.95 | ROL.L | Rolandic_Oper_L |
| 18 | 52.65 | -6.25 | 14.63 | ROL.R | Rolandic_Oper_R |
| 19 | -5.32 | 4.85 | 61.38 | SMA.L | Supp_Motor_Area_L |
| 20 | 8.62 | 0.17 | 61.85 | SMA.R | Supp_Motor_Area_R |
| 21 | -8.06 | 15.05 | -11.46 | OLF.L | Olfactory_L |
| 22 | 10.43 | 15.91 | -11.26 | OLF.R | Olfactory_R |
| 23 | -4.8 | 49.17 | 30.89 | SFGmed.L | Frontal_Sup_Medial_L |
| 24 | 9.1 | 50.84 | 30.22 | SFGmed.R | Frontal_Sup_Medial_R |
| 25 | -5.17 | 54.06 | -7.4 | ORBsupmed.L | Frontal_Mid_Orb_L |
| 26 | 8.16 | 51.67 | -7.13 | ORBsupmed.R | Frontal_Mid_Orb_R |
| 27 | -5.08 | 37.07 | -18.14 | REC.L | Rectus_L |
| 28 | 8.35 | 35.64 | -18.04 | REC.R | Rectus_R |
| 29 | -35.13 | 6.65 | 3.44 | INS.L | Insula_L |
| 30 | 39.02 | 6.25 | 2.08 | INS.R | Insula_R |
| 31 | -4.04 | 35.4 | 13.95 | ACG.L | Cingulum_Ant_L |
| 32 | 8.46 | 37.01 | 15.84 | ACG.R | Cingulum_Ant_R |
| 33 | -5.48 | -14.92 | 41.57 | DCG.L | Cingulum_Mid_L |
| 34 | 8.02 | -8.83 | 39.79 | DCG.R | Cingulum_Mid_R |
| 35 | -4.85 | -42.92 | 24.67 | PCG.L | Cingulum_Post_L |
| 36 | 7.44 | -41.81 | 21.87 | PCG.R | Cingulum_Post_R |
| 37 | -25.03 | -20.74 | -10.13 | HIP.L | Hippocampus_L |

| Index | X | Y | Z | Abbreviated Name | Name |
|---|---|---|---|---|---|
| 38 | 29.23 | -19.78 | -10.33 | HIP.R | Hippocampus_R |
| 39 | -21.17 | -15.95 | -20.7 | PHG.L | ParaHippocampal_L |
| 40 | 25.38 | -15.15 | -20.47 | PHG.R | ParaHippocampal_R |
| 41 | -23.27 | -0.67 | -17.14 | AMYG.L | Amygdala_L |
| 42 | 27.32 | 0.64 | -17.5 | AMYG.R | Amygdala_R |
| 43 | -7.14 | -78.67 | 6.44 | CAL.L | Calcarine_L |
| 44 | 15.99 | -73.15 | 9.4 | CAL.R | Calcarine_R |
| 45 | -5.93 | -80.13 | 27.22 | CUN.L | Cuneus_L |
| 46 | 13.51 | -79.36 | 28.23 | CUN.R | Cuneus_R |
| 47 | -14.62 | -67.56 | -4.63 | LING.L | Lingual_L |
| 48 | 16.29 | -66.93 | -3.87 | LING.R | Lingual_R |
| 49 | -16.54 | -84.26 | 28.17 | SOG.L | Occipital_Sup_L |
| 50 | 24.29 | -80.85 | 30.59 | SOG.R | Occipital_Sup_R |
| 51 | -32.39 | -80.73 | 16.11 | MOG.L | Occipital_Mid_L |
| 52 | 37.39 | -79.7 | 19.42 | MOG.R | Occipital_Mid_R |
| 53 | -36.36 | -78.29 | -7.84 | IOG.L | Occipital_Inf_L |
| 54 | 38.16 | -81.99 | -7.61 | IOG.R | Occipital_Inf_R |
| 55 | -31.16 | -40.3 | -20.23 | FFG.L | Fusiform_L |
| 56 | 33.97 | -39.1 | -20.18 | FFG.R | Fusiform_R |
| 57 | -42.46 | -22.63 | 48.92 | PoCG.L | Postcentral_L |
| 58 | 41.43 | -25.49 | 52.55 | PoCG.R | Postcentral_R |
| 59 | -23.45 | -59.56 | 58.96 | SPG.L | Parietal_Sup_L |
| 60 | 26.11 | -59.18 | 62.06 | SPG.R | Parietal_Sup_R |
| 61 | -42.8 | -45.82 | 46.74 | IPL.L | Parietal_Inf_L |
| 62 | 46.46 | -46.29 | 49.54 | IPL.R | Parietal_Inf_R |
| 63 | -55.79 | -33.64 | 30.45 | SMG.L | SupraMarginal_L |
| 64 | 57.61 | -31.5 | 34.48 | SMG.R | SupraMarginal_R |
| 65 | -44.14 | -60.82 | 35.59 | ANG.L | Angular_L |
| 66 | 45.51 | -59.98 | 38.63 | ANG.R | Angular_R |
| 67 | -7.24 | -56.07 | 48.01 | PCUN.L | Precuneus_L |
| 68 | 9.98 | -56.05 | 43.77 | PCUN.R | Precuneus_R |
| 69 | -7.63 | -25.36 | 70.07 | PCL.L | Paracentral_Lobule_L |
| 70 | 7.48 | -31.59 | 68.09 | PCL.R | Paracentral_Lobule_R |
| 71 | -11.46 | 11 | 9.24 | CAU.L | Caudate_L |
| 72 | 14.84 | 12.07 | 9.42 | CAU.R | Caudate_R |
| 73 | -23.91 | 3.86 | 2.4 | PUT.L | Putamen_L |
| 74 | 27.78 | 4.91 | 2.46 | PUT.R | Putamen_R |
| 75 | -17.75 | -0.03 | 0.21 | PAL.L | Pallidum_L |
| 76 | 21.2 | 0.18 | 0.23 | PAL.R | Pallidum_R |
| 77 | -10.85 | -17.56 | 7.98 | THA.L | Thalamus_L |
| 78 | 13 | -17.55 | 8.09 | THA.R | Thalamus_R |
| 79 | -41.99 | -18.88 | 9.98 | HES.L | Heschl_L |
| 80 | 45.86 | -17.15 | 10.41 | HES.R | Heschl_R |
| 81 | -53.16 | -20.68 | 7.13 | STG.L | Temporal_Sup_L |
| 82 | 58.15 | -21.78 | 6.8 | STG.R | Temporal_Sup_R |
| 83 | -39.88 | 15.14 | -20.18 | TPOsup.L | Temporal_Pole_Sup_L |
| 84 | 48.25 | 14.75 | -16.86 | TPOsup.R | Temporal_Pole_Sup_R |
| 85 | -55.52 | -33.8 | -2.2 | MTG.L | Temporal_Mid_L |
| 86 | 57.47 | -37.23 | -1.47 | MTG.R | Temporal_Mid_R |
| 87 | -36.32 | 14.59 | -34.08 | TPOmid.L | Temporal_Pole_Mid_L |
| 88 | 44.22 | 14.55 | -32.23 | TPOmid.R | Temporal_Pole_Mid_R |
| 89 | -49.77 | -28.05 | -23.17 | ITG.L | Temporal_Inf_L |
| 90 | 53.69 | -31.07 | -22.32 | ITG.R | Temporal_Inf_R |
| 91 | -36.07 | -66.72 | -28.93 | CRBLCrus1.L | Cerebelum_Crus1_L |
| 92 | 37.46 | -67.14 | -29.55 | CRBLCrus1.R | Cerebelum_Crus1_R |
| 93 | -28.64 | -73.26 | -38.2 | CRBLCrus2.L | Cerebelum_Crus2_L |

| Index | X | Y | Z | Abbreviated Name | Name |
|---|---|---|---|---|---|
| 94 | 32.06 | -69.02 | -39.95 | CRBLCrus2.R | Cerebelum_Crus2_R |
| 95 | -8.8 | -37.22 | -18.58 | CRBL3.L | Cerebelum_3_L |
| 96 | 12.32 | -34.47 | -19.39 | CRBL3.R | Cerebelum_3_R |
| 97 | -15 | -43.49 | -16.93 | CRBL45.L | Cerebelum_4_5_L |
| 98 | 17.2 | -42.86 | -18.15 | CRBL45.R | Cerebelum_4_5_R |
| 99 | -23.24 | -59.1 | -22.13 | CRBL6.L | Cerebelum_6_L |
| 100 | 24.69 | -58.32 | -23.65 | CRBL6.R | Cerebelum_6_R |
| 101 | -32.36 | -59.82 | -45.45 | CRBL7b.L | Cerebelum_7b_L |
| 102 | 33.14 | -63.18 | -48.46 | CRBL7b.R | Cerebelum_7b_R |
| 103 | -25.75 | -54.52 | -47.68 | CRBL8.L | Cerebelum_8_L |
| 104 | 25.06 | -56.34 | -49.47 | CRBL8.R | Cerebelum_8_R |
| 105 | -10.95 | -48.95 | -45.9 | CRBL9.L | Cerebelum_9_L |
| 106 | 9.46 | -49.5 | -46.33 | CRBL9.R | Cerebelum_9_R |
| 107 | -22.61 | -33.8 | -41.76 | CRBL10.L | Cerebelum_10_L |
| 108 | 25.99 | -33.84 | -41.35 | CRBL10.R | Cerebelum_10_R |
| 109 | 0.76 | -38.79 | -20.05 | Vermis12 | Vermis_1_2 |
| 110 | 1.38 | -39.93 | -11.4 | Vermis3 | Vermis_3 |
| 111 | 1.22 | -52.36 | -6.11 | Vermis45 | Vermis_4_5 |
| 112 | 1.14 | -67.06 | -15.12 | Vermis6 | Vermis_6 |
| 113 | 1.15 | -71.93 | -25.14 | Vermis7 | Vermis_7 |
| 114 | 1.15 | -64.43 | -34.08 | Vermis8 | Vermis_8 |
| 115 | 0.86 | -54.87 | -34.9 | Vermis9 | Vermis_9 |
| 116 | 0.36 | -45.8 | -31.68 | Vermis10 | Vermis_10 |

## REFERENCES


[1] Zhitao Ying, Dylan Bourgeois, Jiaxuan You, Marinka Zitnik, and Jure Leskovec. Gnnexplainer: Generating explanations for graph neural networks. *Advances in neural information processing systems*, 32, 2019.

[2] Asim Kumar Debnath, Rosa L Lopez de Compadre, Gargi Debnath, Alan J Shusterman, and Corwin Hansch. Structure-activity relationship of mutagenic aromatic and heteroaromatic nitro compounds. correlation with molecular orbital energies and hydrophobicity. *Journal of medicinal chemistry*, 34(2):786–797, 1991.

[3] Romualdo Benigni and Cecilia Bossa. Structure alerts for carcinogenicity, and the salmonella assay system: a novel insight through the chemical relational databases technology. *Mutation Research/Reviews in Mutation Research*, 659(3):248–261, 2008.

[4] John Ashby and Raymond W Tennant. Definitive relationships among chemical structure, carcinogenicity and mutagenicity for 301 chemicals tested by the us ntp. *Mutation Research/Reviews in Genetic Toxicology*, 257(3):229–306, 1991.

[5] Danilo Bzdok and Andreas Meyer-Lindenberg. Machine learning for precision psychiatry: opportunities and challenges. *Biological Psychiatry: Cognitive Neuroscience and Neuroimaging*, 3(3):223–230, 2018.
